# Supplementary material for: Deep K-SVD Denoising
Source: arXiv:1909.13164 source file (2020-11-18)
Supplement: Supplementary file 1 [file 7-SupMat.tex]

\bigskip

\centerline{\bf\Large Supplementary materials}

% \begin{figure*}[!]
% \centering
% \includegraphics[scale = 0.3]{plane.pdf}
% \caption{Plane}
% \end{figure*}

% \begin{figure*}[!]
% \centering
% \includegraphics[scale = 0.3]{person.pdf}
% \caption{Person}
% \end{figure*}

% \begin{figure*}[!]
% \centerin
% \includegraphics[scale = 0.3]{vase.pdf}
% \caption{Vase}
% \end{figure*}

% \begin{figure*}[!]
% \centering
% \includegraphics[scale = 0.3]{face.pdf}
% \caption{Face}
% \end{figure*}

% \begin{figure*}[!]
% \centering
% \includegraphics[scale = 0.3]{wolf.pdf}
% \caption{Wolf}
% \end{figure*}
